# Supplementary material for: RoomTour3D: Geometry-Aware Video-Instruction Tuning for Embodied Navigation
Source: arXiv:2412.08591 source file (2025-03-19)

(a)

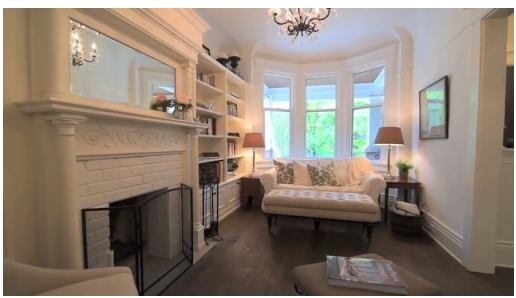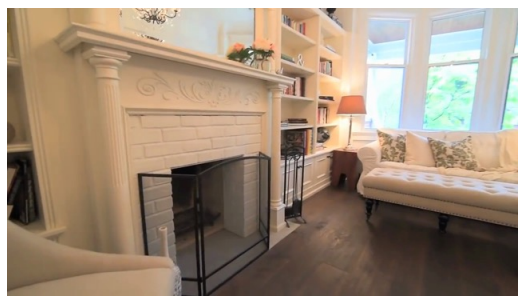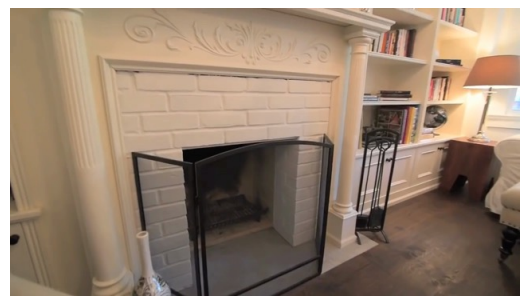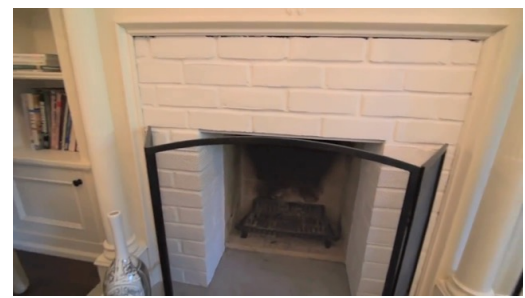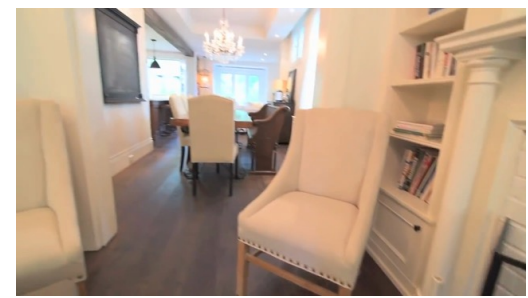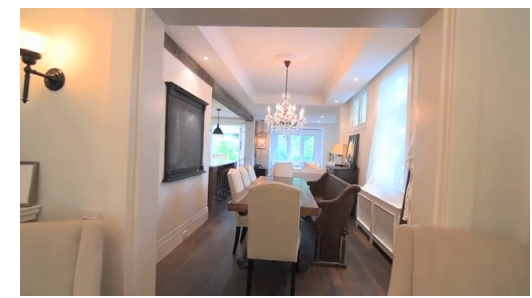

8V1K5RXL2qs, [0169, 0175, 0181, 0187, 0193, 0199]

**Open-end trajectory instruction:**

Navigate through the living room. Begin near an armchair and television, move past a fireplace and gradually approach a bookshelf, continue past pillars, and finally transition into the dining room, approaching a table surrounded by chairs with a chandelier overhead.

(b)

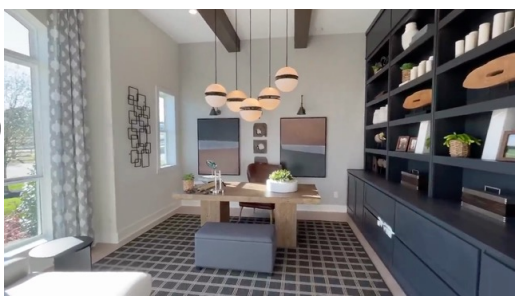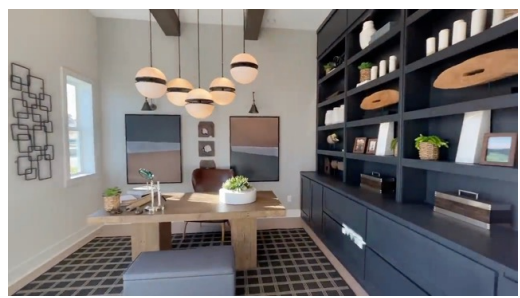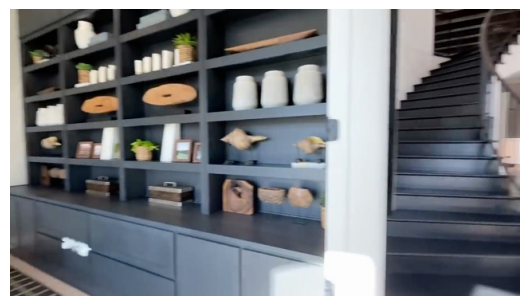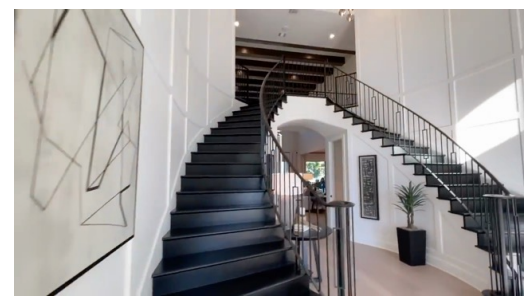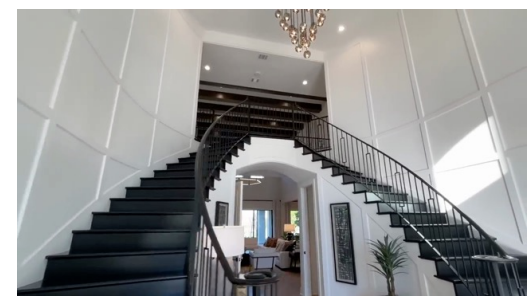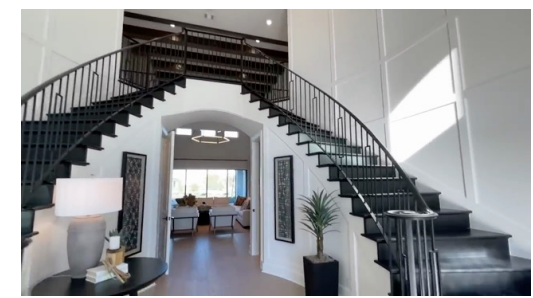

2HCzn1XMKjg, [0200, 0206, 0212, 0218, 0224, 0230]

**Open-end trajectory instruction:**

Navigate through the office. Begin near a cabinet and chairs, pass by a stool and tables, and move towards the living room area, transitioning through the office with various furniture items like bookshelves and drawers. Continue into the hallway, noting a balustrade and stairs, then proceed through the hallway, observing more stairs, balustrades, and chandeliers, before finally arriving at a point with a lamp and room in the distance, indicating a transition to another area.

(c)

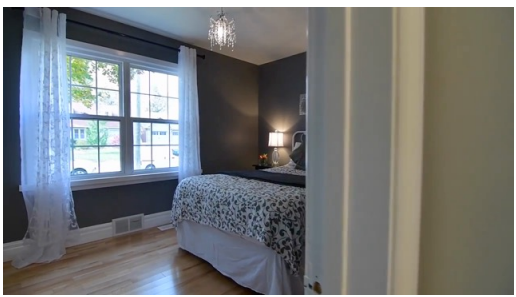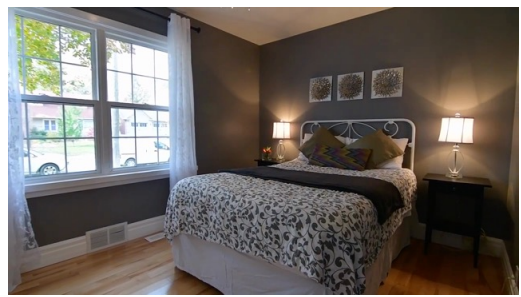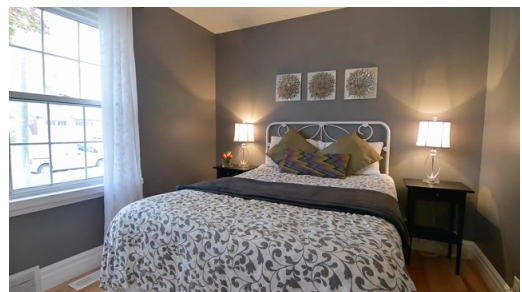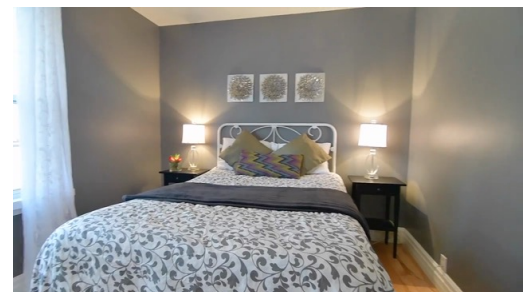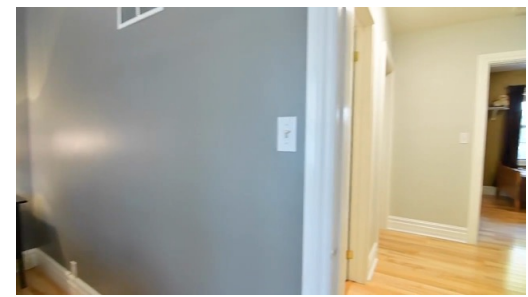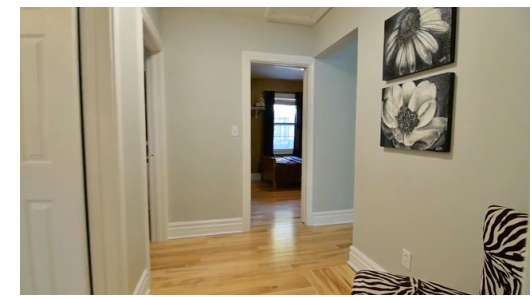

CBsxW0RIIHc, [0409, 0415, 0421, 0427, 0433, 0439]

**Open-end trajectory instruction:**

Navigate through the bedroom. Move forward from the doorway, approach the bed and the far window, veer right past a nightstand and lamp, continue straight toward a closer bed, and finally transition through the doorway into the hallway, passing close to an armchair and art on the right.

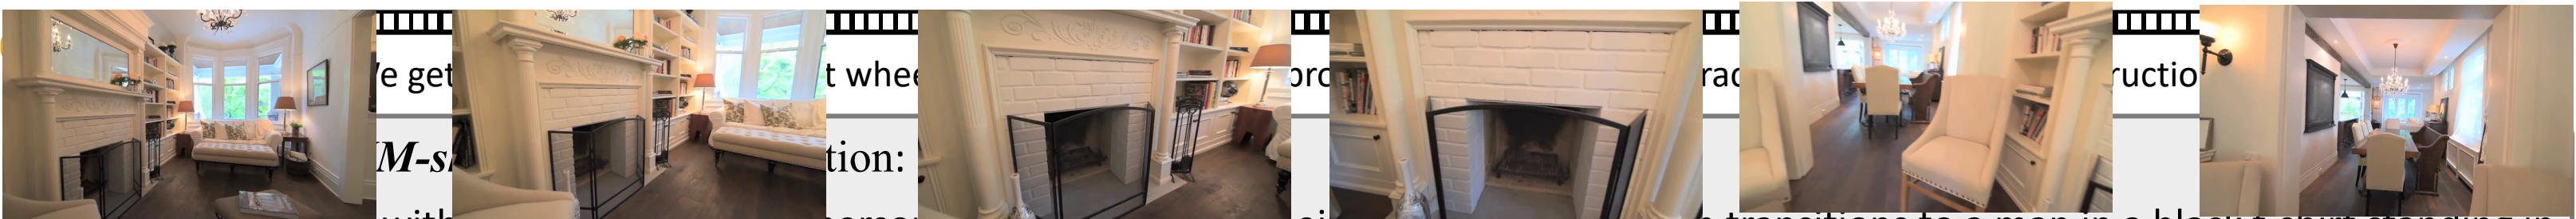

the video begins with a close-up shot of a person holding a pedal in their hand. the scene then transitions to a man in a black t-shirt standing in a garage filled with various items, including a bicycle and a motorcycle. he is engaged in a task at a workbench, where a bicycle is mounted on a stand. as he works, he mentions that he is using a pedal disc for the front wheel. the video then shifts to a wider shot of the man in the black t-shirt, still standing in the garage filled with items. he continues his task at the workbench, where a bicycle is mounted on a stand. the scene then returns to a close-up shot of the man in the black t-shirt, still working at the workbench. the video concludes with a wider shot of the man in the black t-shirt, still standing in the garage filled with items. he continues his task at the workbench, where a bicycle is mounted on a stand.

**Questions:**

- Q1: What are the different components the man handles from the beginning to the end of the video?
- Q2: How does the setting change from the start to the end of the video?
- Q3: What is the man's immediate action after handling the skewer?
- Q4: What is the main activity being depicted in the video?

**Answers:**

- GT1: A pedal, disc brake pad, screws, bell, brackets, skewer, paper, and instruction book.
- GT2: The setting remains the same, in the garage with the half-finished bike.
- GT3: Taking out a piece of paper.
- GT4: The items for the bike assembly or preparation.

**Vicuna answers using summaries & GPT evaluation:**

- A1: The different components the man handles from the beginning to the end of the video are: a piece of equipment, a white object, and the pedals disc for the front wheel. ❌
- A2: The setting changes from a workshop or laboratory to a garage. ❌
- A3: The man is placing the skewer back into the box. ❌
- A4: The main activity being depicted in the video is the demonstration of tool preparation for bikes in a garage setting. ✅

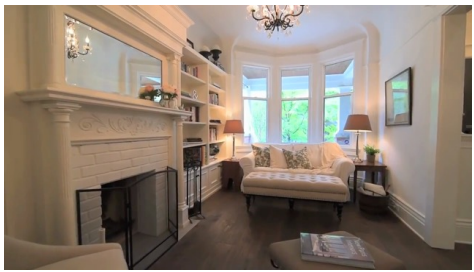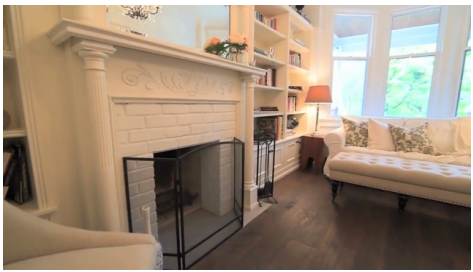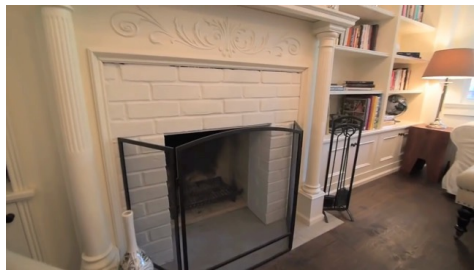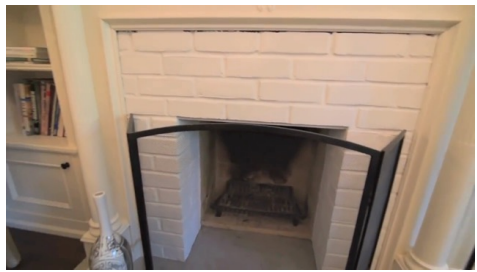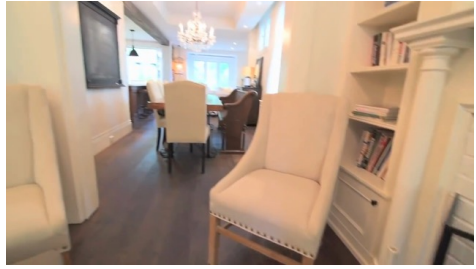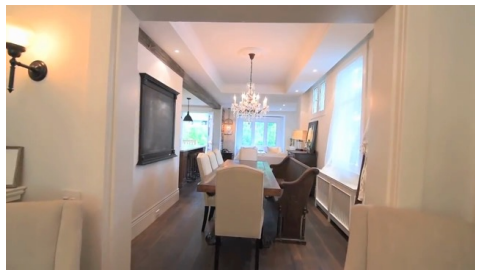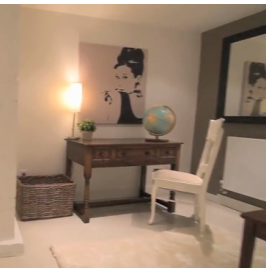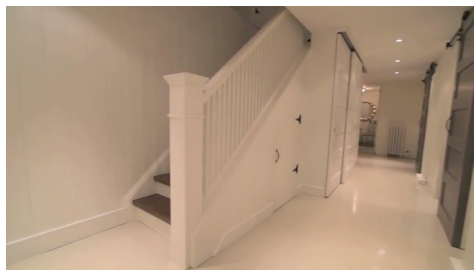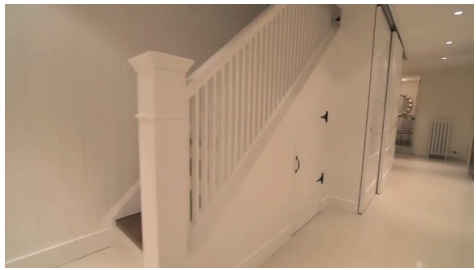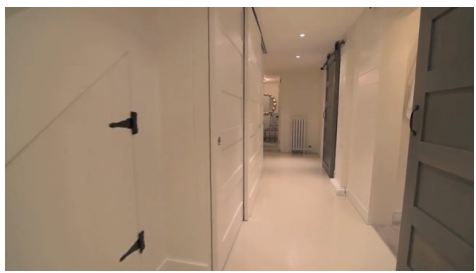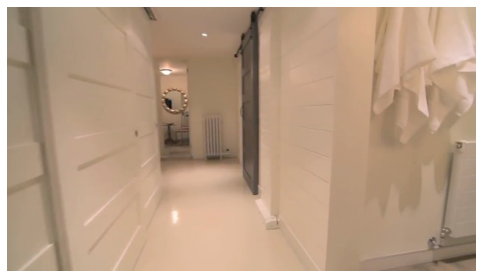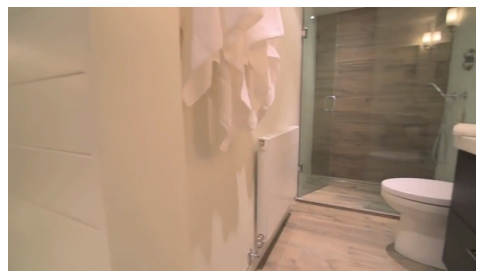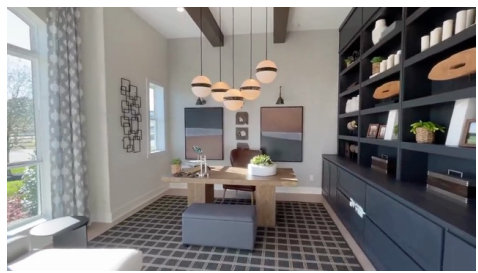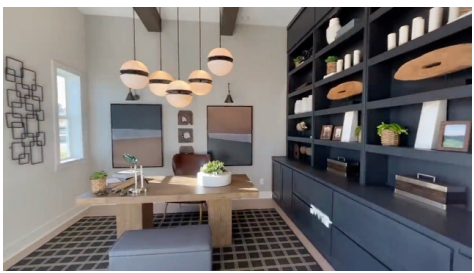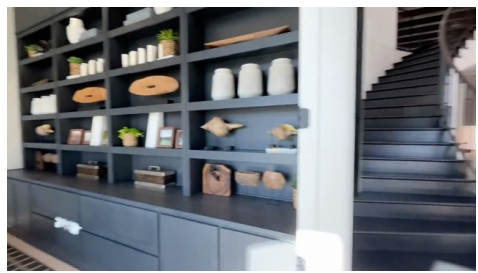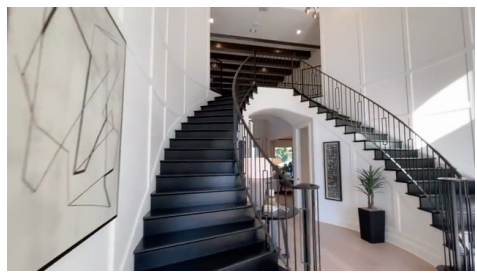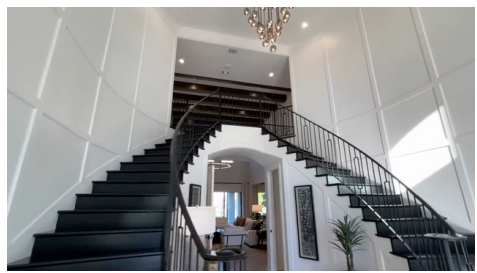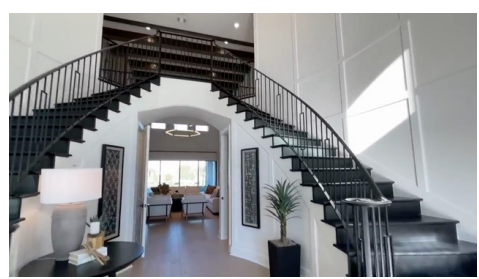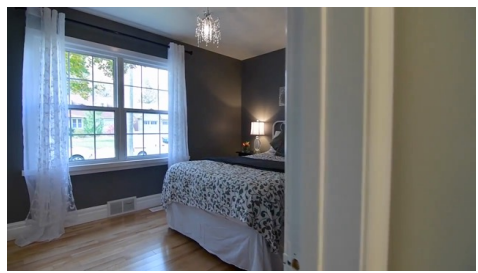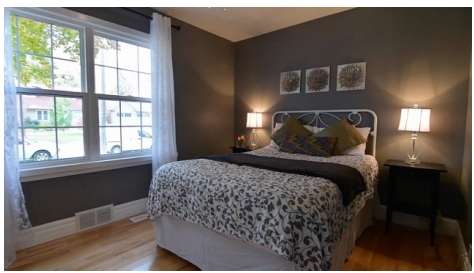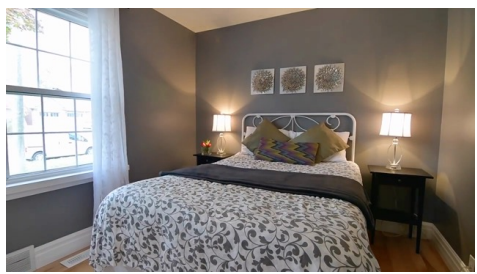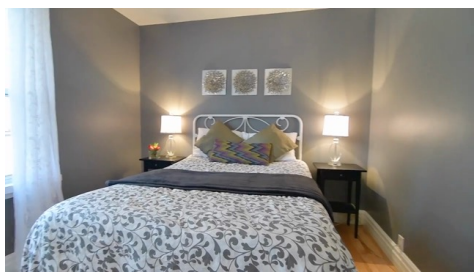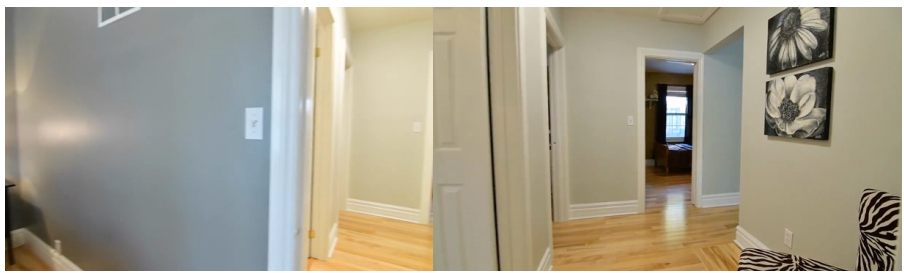

Supplement: Supplementary file 1 [file supp_data_samples.pdf]
