# Supplementary material for: RoomTour3D: Geometry-Aware Video-Instruction Tuning for Embodied Navigation
Source: arXiv:2412.08591 source file (2025-03-19)

You will be given a set of continuous frames. The frames are captured during the camera movement. During movement, the objects in the frames change gradually, like objects passing by, objects moving towards somewhere. You should return a single and concrete sentence describing the camera moving trajectory by the object's progression in the frames. You don't need to mention all the objects. It is good to describe the moving trajectory without all of the objects.

Frames:

\t0: in the study. there is a clock to the right of the current spot in the near distance, a door on left in further distance, a window and curtains in the middle in far distance.

\t1: in the study. there is chair, laptop, table in the middle in the near distance, a door on left in further distance, a window and curtains in the middle in far distance.

\t2: in the study. there is a plant to the left of the current spot in the near distance, wall to the right of the current spot in the near distance, a bench in further distance in the middle, a window and curtains in the middle-right in further distance

Your moving trajectory description: Walk in the study. Move from right to left, pass by a clock to the right of the current spot, approach a table with a chair and laptop, and continue towards a window and curtains in a close distance, approach a plant to the left of the current spot.

Example 2:

Frames:

\t0: In the study. there is a plant, laptop, and table to the left of the current spot in the near distance, a bookshelf to the left of the current spot in the far distance, a door in the middle in further distance, and two art frames to the right of the current spot closely.

\t1: In the study. there is a bookshelf to the left of the current spot in further distance, a door in the middle in further distance, and an art frame in the middle in far distance.

\t2: In the hallway. there is a door to the left of the current spot in the near distance, art frames to the right of the current spot in closer distance

\t3: In the hallway. there is a art frame to the left of the current spot in the near distance, a switch to the right of the current spot in the near distance, a lamp and future stool in the middle in far distance

\t4: In the hallway. there is a wall to the left of the current spot in the near distance, a bed to the left of the current spot in far distance, a wall and lamp and furniture stool in the middle in closer distance.

\t5: In the hallway. there is a wall to the left of the current spot in the near distance, a bed in the middle in closer distance.

\t6: In the bedroom. there is a art frame, plant and furniture stool to the left of the current spot in the near distance, a bed in the middle in the near distance, a window and curtain in a far distance.

Your moving trajectory description: Exit the study. Move from left to right, start near a plant, laptop, and table, pass a bookshelf and approach a door, then shift towards art frames enter the hallway, before move past a switch and approach a lamp and stool, and finally arrive at the bedroom at a bed with a window and curtain in the distance.

Your turn:

Frames:

**{clip\_desc}**

Your moving trajectory description:

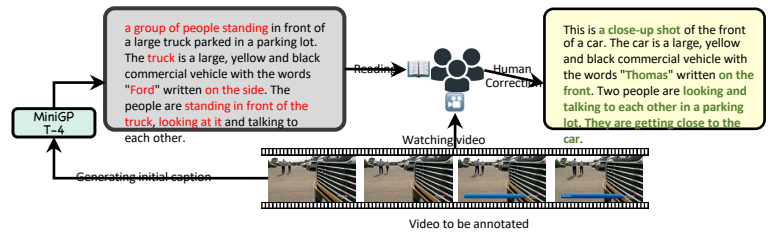

Supplement: Supplementary file 2 [file supp_gpt4_prompt.pdf]
